# Supplementary material for: PLACID: Identity-Preserving Multi-Object Compositing via Video Diffusion with Synthetic Trajectories
Source: arXiv:2602.00267 source file (2026-01-30)
Supplement: Supplementary file 2 [file save_copy.tex]

\clearpage
\setcounter{page}{1}
\maketitlesupplementary


- More on motion-based vs interpolation
- Could show architecture ablations (interpolate vs separate)
- More visualizations
- More details on test set (prompts, visualize)
- More details on training data (examples, prompts)
- Mix identities by conditioning on the wrong object? Or editing examples by changing text?
- Evolution of metrics with inference video length
- inference number of frames vs number of objects?? More objects seem to work better with longer videos
-evolution metrics vs number of objects

\subsection{Training Data Generation}

\paragraph{(i) From In-the-Wild Lifestyle Product Display Images.} All images labeled `Product Photography', `Flat Lay', or `Still‑Life' on Unsplash \cite{unsplash} are parsed together with their captions. For each image we first identify the products being displayed by using the grounding pipeline of Grounding‑DINO \cite{liu2024grounding} together with SAM \cite{kirillov2023segment}, as in \cite{ren2024grounded}. The raw detections are then cleaned by (i) merging detections that share the same label (considering confidence scores and taking the union of their masks), (ii) discarding duplicate masks that carry different labels, (iii) eliminating overlap by subtracting small masks that are wholly or partially contained in larger ones, and (iv) keeping only objects whose mask‑coverage lies between 0.5\% and 80\% of the image area. Images that end up with no valid detections are dropped, and the remaining backgrounds are restored with the inpainting method of \cite{yu2023inpaint}. Each retained object is extracted, randomly reordered, rescaled, and optionally warped with a mild perspective transform; it is then pasted onto a white box to emulate the unsegmented product image $I_i$. To build $F_1$, the first frame of the training video, we scatter these boxed objects across an empty canvas. The canvas background can be (i) plain white, (ii) a randomly chosen background (See \cref{sec:augmentation}), or (iii) the inpainted original background. Finally, a nine‑frame video is rendered: every object travels in a straight line at constant speed from its random start location to its target position in the professional composition, while simultaneously the white boxes fade out and, if a plain‑white background was used initially, the true background fades in. The last frame of the video $F_9$ is thus the desired high‑quality product‑display image, and the intermediate frames provide a temporally coherent progression used for training the model.

\paragraph{(ii) From In-Domain Professionally Designed Compositions.} In-the-wild product‑display images often contain severe occlusions or cut‑off objects, making it impossible to recover their full product appearance. Because faithful detail preservation is essential in our task, we additionally curate a small set of $\sim 400$ manually designed compositions containing the exact kind of layouts, colors, angles, viewpoints and shadows that we aim to generate. For each scene we have (a) the final composition, including background and (b) the separate high‑resolution full image for every displayed object (typically 2–5 items). Using the same pipeline as above, we construct the random‑start frame $F_1$ and synthesize the 9‑frame video, thereby guaranteeing a subset of training data that perfectly matches the target style. The caption paired with each video is created by following one of the pre-computed template prompts that describe the desired transformation and scene, completed with the short description of each individual object and background, which are individually generated using \cite{bai2025qwen2}.


\paragraph{(iii) From 3D-rendered Data.} To teach the model realistic relative scaling and homogeneous illumination we augment the dataset with synthetic 3‑D renders similar to those in \cite{collins2022abo}. From a pool of $\sim 14k$ rendered catalog products we (i) cluster objects into three size groups using K‑Means \cite{mcqueen1967somekmeans}, (ii) select pairs of objects from the same size group, and (iii) place them side‑by‑side on the same imaginary ground plane. Real‑world dimensions are used to scale the objects so that their on‑image size respects the true size ratio (e.g., a product twice as tall appears twice as tall). Both objects share a common lighting setup, corresponding to a soft directional light from the top‑left, ensuring consistent shadows and highlights.
For the initial frame $F_1$, we randomly scatter the unsegmented object images on a randomly chosen background and apply a random relighting (by interpolating several pre‑computed relit versions of the same object). The 9‑frame video is then generated by animating each object from its start location to its final, correctly scaled and illuminated pose, with progressive relighting across frames. Similarly to the previous source, the descriptive caption is built by combining a template with object descriptions generated via \cite{bai2025qwen2}.

\paragraph{(iv) From Subject-Driven Generation Paired Dataset.} Finally, to preserve the text‑image alignment of the pre‑trained I2V model and to encourage plausible object placements (\eg, a laptop on a table, shoes on the floor), we exploit a filtered subset of the Subject‑200k dataset \cite{tan2024ominicontrol}. Each filtered pair consists of (a) a white‑background catalog image of an object and (b) a second image of the same object in a different context, together with a descriptive caption. We discard pairs where the object identity changes, mostly due to one or both images being AI-generated, by running Grounding‑DINO \cite{liu2024grounding} with the same object description on each pair and keeping only those where each object description yields a bounding box with confidence $>0.55$ in both images. For each pair, the image with white background is used as $F_1$ and the other one is the last frame of a 9‑frame video. In this case, however, since significant reposes of the target object between $F_1$ and $F_9$ are possible, an identity preserving physical transformation of the object from one frame to the other is not possible. Therefore, the video is built via interpolation of the two frames, and the training objective is adapted to only take into account the last frame instead of the entire video.

\subsection{Training Data Augmentations}
\label{sec:augmentation}

Collectively, the four data pipelines in \cref{sec:data} provide a large, richly annotated set of (background, object images, target composition, transition video, caption) tuples that enable our model to learn the full transformation from a random, unsegmented layout to a high‑fidelity, caption‑driven multi-product display. This data is paired with different kinds of augmentations to extend the model's usability and further encourage visual diversity and robustness.

%While the training data described in \cref{sec:data} provides all the needed information for generating realistic and aesthetic compositions of products, there are some simple augmentations that can be applied to the training data for extending the model's use to more diverse applications. 

\paragraph{Object Augmentation.} To discourage the model from simply copying the objects from the supplied images $I_{1..N}$, during training, each object is randomly (i) rescaled, (ii) rotated, and (iii) applied a small perspective warping. The resulting object images are scattered around the unchanged background in randomized order to avoid any rearrangement biases, while ensuring all objects are fully present in the image and there is no overlap between them. %For discourage copy-paste behaviour of objects from their provided images $I_i$, during training, each object is randomly (i) rescaled, (ii) rotated, and (iii) applied a small perspective warping. The resulting object images are scattered around the unchanged background in randomized order, while ensuring all objects are fully present in the image and there is no overlap between them.

\paragraph{Background Augmentation.} To make the model resilient to a wide variety of background textures, each training iteration that uses a random background, draws it at random from one of three pools: (i) a collection of high‑quality background photos that match the aesthetic typically used by professional designers, (ii) a plain background filled with a randomly sampled RGB colour, and (iii) backgrounds created on the fly by combining simple primitives such as linear gradients, block textures, or radial gradients with harmonious colour palettes. By mixing these three sources during training, the network learns to operate equally well on simple solid colours, patterned textures, and realistic photographic backdrops, thereby improving its robustness to any background it may encounter at test time.

%To increase robustness to different backgrounds, with simple or more complex textures and patterns, every time a random background is used during training, it is picked from one of three sources: (i) sampled from a bank of designer-approved images similar to those they typically use, (ii) generated as a plain background of an aleatory picked RGB color, or (iii) automatically generated by using a linear gradient, block pattern on radial gradient, combining different harmonious colors.


\paragraph{Scene Completion.} During training we randomly apply a “scene‑completion’’ augmentation with a $20\%$ probability. In such cases the selected objects are treated as part of the background: their final positions are incorporated into the background description of the caption, and the background image (if one is provided) is edited to contain those objects throughout the entire 9‑frame video. The remaining objects are still supplied as explicit conditioning inputs and are animated from their initial random locations to their target poses; they may even be partially occluded by the newly added background objects. This augmentation encourages the model to handle both foreground objects and items that naturally belong to the scene, improving robustness to varied compositional scenarios. %With a probability of 20\%, we set each object to be part of the background. Therefore, the product description gets added to the background description in the caption, and the provided background image, if existing, is updated to include those objects in their final location throughout the 9-frame video. The rest of the objects are added as conditioning objects, being animated into their respective location, and even having `background' objects overlapping on them if necessary.

\paragraph{Design Elements.} With probability $10\%$ we treat a conditioning object as a design element rather than as an explicit visual cue. In that training step the object’s image $I_i$ is omitted from the visual conditioning set and does not appear in the initial frame of the video. Its description is inserted only in the caption $c$ (outside any $<OBJ> … </OBJ>$ block). During video synthesis the object ``flies in'' from outside the frame and reaches its target pose in the final frame. This forces the model to rely on the textual description alone for that item, encouraging robust text‑driven placement and improving generalisation to unseen design elements. %With a probability of 10\%, each conditioning object is considered as a `design element'. Therefore, their image $I_i$ is not provided as conditioning in that training step, and they don't appear in any form in the first frame of the video. Instead, their description is added as part of the caption $c$, without being included in any object's description, and they fly into their final location in the training video from outside the frame.

\paragraph{Object Replacement.} To enable the model to edit existing scenes or reuse predefined layouts, we introduce a replacement augmentation. When none of the objects in a training sample are designated as background elements or design‑only elements, we (with probability $7\%$) select one object and substitute it with a new product. The replacement inherits the original object’s position, scale, and relighting. Simultaneously, the caption is updated to describe the substitution so that the transformation is reflected consistently throughout the nine‑frame video. This augmentation teaches the model to seamlessly swap items while preserving the overall composition. %For allowing the model to edit existing scenes, or copy layouts of pre-designed scenes, when none of the objects are considered as part of the background nor as design elements, with a probability of 20\%, an object is considered as part of the background will be replaced for a new one. In this case, the new object inherits the location of the previously existing object, as well as any transformation such as rotation, rescaling or relighting. The descriptive caption is simultaneously updated to reflect the new change happening throughout the video.
